# Supplementary material for: Reductions for Safety Proofs (Extended Version)
Source: arXiv:1910.14619 source file (2019-10-31)
Supplement: Supplementary file 1 [file appendix.tex]

%!TEX root = ./popl20.tex
\begin{toappendix}
\section{Benchmarks}\label{app:benchmarks}

\begin{table}[h!]
\centering
{\scriptsize
\begin{tabular}{|l|l|}\hline
  Benchmark & Description \\ \hline
  \hline
  channel-sum                  &  One thread computes a queue some and another thread modifies it. \\
  commit-1-alt                 &  A commit protocol between a client, manager, and 1 node. \\
  commit-2-alt                 &  A commit protocol between a client, manager, and 1 node. \\
  nonblocking-counter          &  Similar to example from Figure \ref{fig:me1} with a non-blocking decrement.  \\
  nonblocking-counter (alt)    &  The above example with a different pre/post-condition.\\
  Figure \ref{fig:me1}         &  Example of Figure \ref{fig:me1} \\
  counter-alt                  &  Example of Figure \ref{fig:me1} with a different pre/post-condition. \\
  counter-determinism          &  Four-threaded instance to prove Example of Figure \ref{fig:me1} is deterministic. \\
  counter-fun                  &  Iterated application of an uninterpreted function and its inverse. \\
  Figure \ref{fig:me2}         &  Example of Figure \ref{fig:me2}. \\
  mult-4                       &  4-threaded version of the example from Figure \ref{fig:me2}. \\
  difference-det               &  Determinism of a two-threaded subtraction function. \\
  horseshoe                    &   3 threads communicating over queues and computing 3 values collaboratively.\\
  mult-equiv                   &  Equivalence of a single and a double threaded multiplication routines.\\
  prod-consumer                &  Producer-consumer communicating through a queue and incrementally transferring a counter value. \\
  prod-consumer-3              &  The three-threaded version of the above. \\
  prod-consumer-equiv          &  Equivalence of a producer-consumer program to its sequential version. \\
  queue-add-2                  &  One thread sends numbers to another to add. \\
  queue-add-3                  &  Same as above, with an extra thread in between. \\
  send-receive                 &  One thread alternates between sending two values to another thread. \\
  send-receive-alt             &  Same as above, with a post-condition instead of an assert in a monitor thread. \\
  simple-array-sum             &  3-threaded program summing an array with constants into a new array. \\
  simple-queue                 &  Example of Figure \ref{fig:eb1}.\\
  threaded-sum-3               &  3-threaded program doing a coordinated element-wise sum of two arrays with timing.\\
  three-array-max              &  3-threaded program comparing the max of element-wise added arrays and their individual maxs.\\
  three-array-min              &  3-threaded program comparing the min of element-wise added arrays and their individual mins.\\
  three-array-sum              &  3-threaded program comparing the sum of element-wise added arrays and their individual sums.\\
  two-queue                    &  2 loops concurrently swap their counters via queues. \\\hline
\end{tabular}
}
\caption{A list of benchmarks and their short descriptions.}
\end{table}

\end{toappendix}
